# Supplementary material for: Flavour Condensate and the Dark Sector of the Universe
Source: arXiv:1202.3812 source file (2012-02-16)
Supplement: Supplementary file 1 [file dimreg.tex]

\section{Dimensional Regularization}

In this section we explore a first na\"ive attempt on renormalizing the theory: we will
remove ``by hand'' infinities present in the expression $\lfv :T_{\mu\nu}(x): \rfv$.
More specifically, we have that
\be
\lfv :T_{\mu\nu}(x): \rfv=\int d\vk \mathcal{T} (k)
\ee
with ultraviolet divergences present on the right hand side (for sake of clarity, we will omit tensorial indices, being understood
in all expressions).
In order to remove them, we consider
\be
\int d\vk \mathcal{T}(k)=\Omega_D\int d k\;k^{D-1} \mathcal{T}(k)\Big|_{D=3}.
\ee
with $\Omega_D$ the solid angle of dimension $D$
The latest integral is ill defined for $D=3$, but it might be possible to solve it for other values of $D$.
We then regard at a generic solution of
\be
\Omega_D\int d k\;k^{D-1} \mathcal{T}(k)
\ee
as a function of $D\in\field{C}$:
\be
\Omega_D\int d k\;k^{D-1} \mathcal{T}(k)\equiv\mathfrak{T}(D)\;\;\;\;\;\;\;\;D\in A\subset\field{C}.
\ee
with $A$ a region on the complex plane on which $\mathfrak{T}(D)$ is well-behaved.
Such a function is obviously ill-defined for $D=3$, and it might also present other poles on the complex plane.
We then consider the expansion in series of $\mathfrak{T}(D)$ around $D=3$ that would give us:
\be
\mathfrak{T}(D)=...+\frac{t_{-2}}{(D-3)^2}+\frac{t_{-1}}{(D-3)}+t_0+t_1 (D-3)+t_2 (D-3)^2+....
\ee
In our renormalization scheme we will remove the divergent terms and we will consider only finite terms of the
above series, in the limit $D\rightarrow3$:
\be
\mathfrak{T}^{rin}(D)\equiv \mathfrak{T}(D)-\frac{t_{-1}}{(D-3)}-\frac{t_{-2}}{(D-3)^2}-...
\ee
and therefore
\be
\lfv T^{rin}(x) \rfv \equiv  \lim_{D\rightarrow3}\mathfrak{T}^{rin}(D)=t_0.
\ee
We shall now implement this method on the explicit quantities for the energy and the pressure.
Unfortunately, as we will see, the expression for the energy turns out to be dimensionally not well-defined.

\begin{center}
PRESSURE
\end{center}
Since
\be
\lfv : T_{jj}(x):\rfv =-\sst \frac{m_1^2-m_2^2}{2}\int \frac{d^3p}{(2 \pi)^{3}}\left(\frac{1}{ \w_2(p)}-\frac{1}{ \w_1(p)}\right)
\ee
we have
\be
-\sst \frac{m_1^2-m_2^2}{2}\int \frac{d^dp}{(2 \pi)^{3}}\left(\frac{1}{ \w_2(p)}-\frac{1}{ \w_1(p)}\right)=\nonumber
\ee
\be
\frac{1}{2} \Omega _d \left(m_1^2-m_2^2\right) \sin
   ^2(\theta )\int^{\infty}_0 dk \frac{k^{d-1}
   \left(\frac{1}{\sqrt{k^2+m_1^2}}-\frac{1}{\sqrt{k^2+m_2^2
   }}\right)}{8 \pi ^3}=
\ee
\be
	=-\frac{\Gamma \left(\frac{1}{2}-\frac{d}{2}\right) \Gamma
   \left(\frac{d}{2}\right) \Omega _d
   \left(m_1^2-m_2^2\right) \sin ^2(\theta ) \left(m_1
   m_2^d-m_2 m_1^d\right)}{32 \pi ^{7/2} m_1
   m_2}=
\ee
\be
		\frac{ \Omega _d\left(m_1^2-m_2^2\right)^2 \sin ^2(\theta )}{32 \pi ^3
   (d-3)}-\frac{ \Omega _d \sin ^2(\theta ) }{64 \pi ^3}(m_1-m_2) (m_1+m_2)\cdot\nonumber
\ee
\be
		\cdot\left(
   (\log (4)-1) (m_1-m_2) (m_1+m_2)+2
    \log \left(\frac{m_2^{m_2^2}}{m_1^{ m_1^2}}\right)\right)+\nonumber
\ee
\be
+\mathcal{O}(d-3)
\ee
and therefore
\be
\lfv T_{jj}^{rin}(x)\rfv=-\frac{  \sin ^2(\theta ) }{16 \pi ^2}(m_1-m_2) (m_1+m_2)\cdot\nonumber
\ee
\be
		\cdot\left(
   (\log (4)-1) (m_1-m_2) (m_1+m_2)+2
    \log \left(\frac{m_2^{m_2^2}}{m_1^{ m_1^2}}\right)\right)=\nonumber
\ee
\be
=-\frac{ \sin ^2(\theta ) }{16 \pi ^2}\left((\log (4)-1)(m_1^2-m_2^2)^2+2(m_1^2-m_2^2) \log \left(\frac{m_2^{m_2^2}}{m_1^{ m_1^2}}\right)\right)
\ee
with $\log (4)-1\approx 0.386$.

\begin{center}
ENERGY
\end{center}
Since
\be
\lfv : T_{00}(x):\rfv =\sst \frac{(m_1-m_2)^2}{2}\int \frac{d^3p}{(2 \pi)^{3}}\left(\frac{1}{ \w_2(p)}+\frac{1}{ \w_1(p)}\right)
\ee
we have
\be
\sst \frac{(m_1-m_2)^2}{2}\int \frac{d^dp}{(2 \pi)^{3}}\left(\frac{1}{ \w_2(p)}+\frac{1}{ \w_1(p)}\right)=\nonumber
\ee
\be
=\frac{\Omega _d \Gamma \left(\frac{1}{2}-\frac{d}{2}\right) \Gamma
   \left(\frac{d}{2}\right) (m_1-m_2)^2 \sin ^2(\theta )
   \left(m_2 m_1^d+m_1 m_2^d\right)}{16 \pi
   ^{7/2} m_1 m_2}=\nonumber
\ee
\be
=\frac{\Omega _d (m_1-m_2)^2 (m_1^2+m_2^2) \sin ^2(\theta )}{16 \pi ^3 (d-3)}+
\ee
\be
-\frac{\Omega _d  \sin ^2(\theta )
   }{32 \pi ^3}(m_1-m_2)^2\left((\log (4)-1) (m_1^2+m_2^2)-2  \log (m_2^{m_2^2} m_1^{m_1^2})\right)+\mathcal{O}\left((d-3)^1\right)
\ee
and therefore
\be
\lfv T_{00}^{rin}(x)\rfv =-\frac{ \sin ^2(\theta )
   }{8 \pi ^2}(m_1-m_2)^2\left((\log (4)-1) (m_1^2+m_2^2)-2  \log (m_2^{m_2^2} m_1^{m_1^2})\right)
\ee
Such an expression is not well defined dimensionally, because of the term $ \log(m_2^{m_2^2} m_1^{m_1^2})$ coming from
\be
\partial_d m_1^d=\partial_d e^{d\log (m_1)}=\log( m_1)e^{d\log (m_1)}=\log(m_1)m_1^d.
\ee
